# Supplementary material for: Self-synchronization of Kerr-nonlinear Optical Parametric Oscillators
Source: arXiv:1602.08523 ancillary file (2016-02-26)
Supplement: Supplementary file 1 [file phase_locking_SM.pdf]

# Supplemental Material to
# Self-synchronization of Kerr-nonlinear Optical Parametric Oscillators

H. Taheri[a], P. Del'Haye[b], A. A. Eftekhar[a], K. Wiesenfeld[c], A. Adibi[a]

[a]*School of Electrical and Computer Engineering, Georgia Institute of Technology, Atlanta, GA, USA*
[b]*National Physical Laboratory, Teddington, United Kingdom*
[c]*Center for Nonlinear Science, School of Physics, Georgia Institute of Technology, Atlanta, GA, USA*

## Fourier transform definition, the magnitude and phase equations

The intra-cavity field envelope $\psi(\theta,\tau)$ and the complex-valued comb teeth amplitudes $\tilde{a}_\eta(\tau)$, $\eta \in \{0, \pm1, \pm2, \pm3, \dots, \pm N\}$, are Fourier transform pairs related through the following equations

$$\psi(\theta,\tau) = \sum\nolimits_{\eta=-N}^{N} \tilde{a}_\eta(\tau)\exp(+\mathrm{i}\eta\theta), \tag{SM.1.a}$$

$$\tilde{a}_\eta(\tau) = \frac{1}{2\pi}\int_{-\pi}^{\pi} \mathrm{d}\theta\ \psi(\theta,\tau)\exp(-\mathrm{i}\eta\theta). \tag{SM.1.b}$$

Using these relations and exploiting $\int_{-\pi}^{\pi}\mathrm{d}\theta\ \exp[\mathrm{i}(\eta-\eta')\theta] = 2\pi\delta_{\eta\eta'}$, it is straightforward to find the equivalent coupled nonlinear ordinary differential equations (NODEs) from the LLE. The result is

$$\frac{\mathrm{d}\tilde{a}_\eta}{\mathrm{d}\tau} = \tilde{F}_\eta - (1+\mathrm{i}\alpha)\tilde{a}_\eta + \mathrm{i}\frac{d_2}{2}\eta^2\tilde{a}_\eta + \mathrm{i}\sum_{l,m,n}\tilde{a}_l\tilde{a}_m^*\tilde{a}_n\delta_{\eta_{lmn}\eta}, \tag{SM.2}$$

where $\delta_{pq}$ is the Kronecker delta (for integers $p$ and $q$), $\eta_{lmn} = l - m + n$, and $\tilde{F}_\eta(\tau)$ is the Fourier transform of $F$ and is equal to $\delta_{0\eta}F_\mathrm{P}\exp(\mathrm{i}\phi_\mathrm{P})$ for a CW pump. In the strong pumping regime and exploiting the symmetry of the power spectrum, it is straightforward to separate the magnitude and phase equations to get

$$\begin{aligned}\frac{\mathrm{d}}{\mathrm{d}\tau}\ln(a_\eta) \\ &= -1 + \frac{a_{-\eta}}{a_\eta}{a_0}^2\sin(\phi_\eta+\phi_{-\eta}-2\phi_0) + \frac{1}{a_\eta}F_\mathrm{P}\cos(\phi_\mathrm{P}-\phi_\eta)\,\delta_{0\eta} \\ &\quad - \frac{a_0}{a_\eta}\sum_l a_l\{2a_{\eta+l}\sin(\phi_0-\phi_l+\phi_{\eta+l}-\phi_\eta) + a_{\eta-l}\sin(\phi_l-\phi_0+\phi_{\eta-l}-\phi_\eta)\},\end{aligned}$$

and

$$\dot{\phi}_\eta = 2a_0^2 - \alpha + \frac{1}{2}d_2\eta^2 + \frac{a_{-\eta}}{a_\eta}{a_0}^2\cos(2\phi_0 - \phi_\eta - \phi_{-\eta}) + \frac{1}{a_\eta}F_\mathrm{P}\sin(\phi_\mathrm{P} - \phi_\eta)\,\delta_{0\eta}$$
$$+ \frac{a_0}{a_\eta}\sum_l a_l\{2a_{\eta+l}\cos(\phi_0 - \phi_l + \phi_{\eta+l} - \phi_\eta) + a_{\eta-l}\cos(\phi_l - \phi_0 + \phi_{\eta-l} - \phi_\eta)\}.$$

Using the phase equation, the equations of motion for the centered phase averages $\zeta_\eta = (\phi_\eta + \phi_{-\eta})/2 - \phi_0$ and phase differences $\Delta_\eta = (\phi_\eta - \phi_{-\eta})/2$ are readily found,

$$\dot{\zeta}_\eta = \frac{1}{2}d_2\eta^2 + a_0^2\{1 + \cos(-2\zeta_\eta)\} - \frac{1}{a_0}F_\mathrm{P}\sin(\phi_\mathrm{P} - \phi_0)$$
$$+ \frac{a_0}{a_\eta}\sum_l a_l a_{\eta-l}\cos(\Delta_l + \Delta_{\eta-l} - \Delta_\eta)\,\{2\cos(\zeta_{\eta-l} - \zeta_\eta - \zeta_l) + \cos(\zeta_{\eta-l} - \zeta_\eta + \zeta_l)\},$$

$$\dot{\Delta}_\eta = \frac{a_0}{a_\eta}\sum_{l=-(N-\eta)}^{N} a_l a_{\eta-l}\{2\sin(\zeta_\eta - \zeta_{\eta-l} + \zeta_l) + \sin(\zeta_\eta - \zeta_{\eta-l} - \zeta_l)\}\sin(\Delta_l + \Delta_{\eta-l} - \Delta_\eta).$$

The magnitude and phase equations for the pumped mode

$$\frac{\mathrm{d}}{\mathrm{d}\tau}\ln(a_0) = \frac{F_\mathrm{P}}{a_0}\cos(\phi_\mathrm{P} - \phi_0) - 1,$$
$$\dot{\phi}_0 = \frac{F_\mathrm{P}}{a_0}\sin(\phi_\mathrm{P} - \phi_0) - \alpha + {a_0}^2.$$

include no linear contributions from $a_{\eta\neq 0}$ (corrections are proportional to $a_\eta^2$, $\eta \neq 0$), and their solutions yield the equilibrium intra-cavity field $\psi_\mathrm{e} = a_0\exp(\mathrm{i}\phi_0)$. It is worth noting that $|\psi_\mathrm{e}|$ can also be found from solving the cubic equation resulting from setting the temporal and spatial derivatives equal to zero in the LLE.

## Dispersion and the effect of higher-order coefficients

The resonance frequencies of a microresonator can be expanded as a Taylor series in the mode number $\eta$ and at the pumped resonance $\omega_0$, namely,

$$\omega_\eta = \omega_0 + D_1\eta + \frac{1}{2!}D_2\eta^2 + \frac{1}{3!}D_3\eta^3 + \cdots.$$

The modes are counted with respect to the pumped resonance, such that the pumped resonance has mode number $\eta = 0$ and frequency $\omega_0$. In this series expansion, $D_1$ is the free-spectral range (FSR), and $D_j$, $j \geq 2$, are the $j$-th order dispersion coefficients. These coefficients are related to the $\beta_j$ coefficients in the expansion $\beta(\omega) = \beta_0 + \beta_1\omega + \frac{1}{2!}\beta_2\omega^2 + \frac{1}{3!}\beta_3\omega^3 + \cdots$, of the propagation constant in frequency, through

$$\beta_1 = \frac{n}{c} = \frac{1}{D_1 R},$$
$$\beta_2 = -\frac{D_2}{D_1^2}\beta_1,$$
$$\beta_3 = -\frac{3D_2}{D_1^2}\beta_2 - \frac{D_3}{D_1^3}\beta_1,$$

$$\beta_4 = -\frac{4D_2}{D_1^2}\beta_3 - \frac{6D_3}{D_1^3}\beta_2 - \left(\frac{3D_2^3}{4D_1^6} + \frac{D_4}{D_1^4}\right)\beta_1.$$

Here, $n$ is the effective refractive index of the microresonator at the pumped resonance frequency and $c$ is the speed of light. Using these expressions, one can convert the $D_j$ coefficients to $\beta_j$'s or vice versa. Although for clarity of the argument we have excluded dispersion coefficients beyond $d_2 = -2D_2/\Delta\omega_0$ in our analysis, they can be included in the model so long as $|d_j| = |2D_j/\Delta\omega_0| \ll 1$. For instance, in the presence of the third-order dispersion coefficient, Eq. (4) of the main text becomes

$$\dot{\Delta}_\eta = \frac{d_3}{6}\eta^3 + \frac{a_0}{a_\eta}\sum\nolimits_{l=-(N-\eta)}^{N} K(l,\eta)\sin(\Delta_l + \Delta_{\eta-l} - \Delta_\eta). \qquad \text{(SM.3)}$$

In typical optical microresonators used for soliton formation (e.g., silicon nitride or magnesium fluoride), $|d_3| = |2D_3/\Delta\omega_0| \approx 10^{-5}$. With higher order dispersion coefficients, the symmetry of the comb magnitudes with respect to the pumped mode would not hold anymore, yet in numerical integrations of the above equation phase steps close to $\pi$ are still observed in the steady-state. An example is shown in Fig. (SM1) for $|d_3| = 0.0001$.

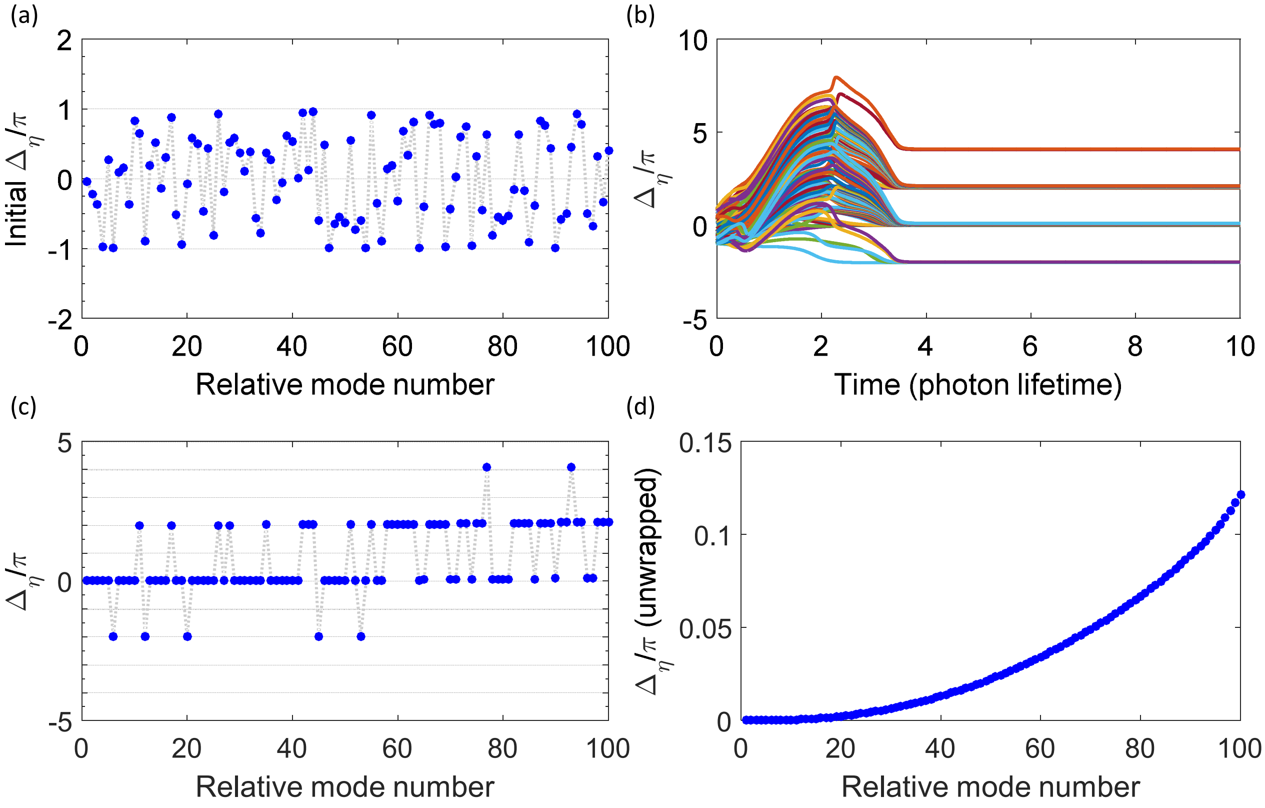


Fig. SM1. Integration of Eq. (SM.3) for a comb with 201 teeth and $|d_3| = |2D_3/\Delta\omega_0| = 0.0001$. (a) Initial values of the phase differences. (b) Temporal evolution of the phase differences. (c) Steady-state phase differences. (d) Unwrapped values of the steady-state phase differences. The steady-state phase differences are approximately equal to integer multiples of $\pi$.

## Modulational instability gain profile and comb generation threshold

Comb generation threshold can be found simply by writing $\psi(\theta,\tau)=\tilde{a}_0+\ \delta\psi(\theta,\tau)$ (where $\tilde{a}_0=\tilde{a}_{0,\mathrm{SS}}$ is the complex-valued equilibrium intra-cavity field), and linearizing the LLE in the perturbation $\delta\psi(\tau)$. The result, after projecting on the cavity modes, is a 3-mode model with the following equations [SM1,SM2]

$$\frac{\mathrm{d}}{\mathrm{d}\tau}\begin{bmatrix} a_\eta \\ a^*_{-\eta}\end{bmatrix}=\begin{bmatrix} P & Q \\ Q^* & P^*\end{bmatrix}\begin{bmatrix} a_\eta \\ a^*_{-\eta}\end{bmatrix}\cdot$$

with

$$P=\ -1+\mathrm{i}\left[2{a_0}^2-\left(\alpha-\frac{1}{2}d_2\eta^2\right)\right],$$

$$Q=\mathrm{i}{a_0}^2\cdot$$

The eigenvalues for the matrix of coefficients are

$$\lambda_\pm=-1\pm\sqrt{{a_0}^4-\left(\alpha-\frac{1}{2}d_2\eta^2-2{a_0}^2\right)^2}\cdot$$

For the perturbation to grow with time, the eigenvalues should have positive real parts. For that to happen, the following inequalities should hold,

$${a_0}^2\geq\left|\alpha-\frac{1}{2}d_2\eta^2-2{a_0}^2\right|, \tag{SM.4}$$

$${a_0}^4-\left(\alpha-\frac{1}{2}d_2\eta^2-2{a_0}^2\right)^2\geq 1\cdot \tag{SM.5}$$

The second of these inequalities guarantees the first one. Mode numbers $\eta$ for which $\mathrm{Re}\{\lambda_+\}>0$ have the chance to grow with time and $\Gamma(\eta)=\mathrm{Re}\{\lambda_+\}$ is the modulational instability (MI) gain parameter. The comb tooth number for MI gain peak is the nearest integer to $\sqrt{2(\alpha-2a_0^2)/d_2}$. We note that $\mathrm{Re}\{\lambda_-\}>0$ cannot hold for any set of parameters $\alpha$, $d_2$, $a_0$, and $\eta$, since whether the expression under the square root in $\lambda_-$ is positive or negative, $\mathrm{Re}\{\lambda_-\}$ will be negative. The second inequality above can be written as

$${a_0}^4-1\geq\left(\alpha-\frac{1}{2}d_2\eta^2-2{a_0}^2\right)^2\geq 0\cdot$$

${a_0}^4-1\geq 0$ shows that $a_0=1=\left|a_{0,\mathrm{Th}}\right|$ is the comb generation threshold. The mode numbers $\eta$ which satisfy the above inequality at threshold [SM1] are $\eta_{\mathrm{Th}}=\pm[2(\alpha-2)/d_2\ ]^{1/2}$.

## The equation for early temporal evolution of the centered phase averages: phase anti-symmetrization

The equation for the temporal evolution of $\zeta_\eta$ is

$$\dot{\zeta}_\eta = -\frac{1}{a_0} F_\mathrm{P} \sin(\phi_\mathrm{P} - \phi_0) + \frac{1}{2} d_2 \eta^2 + a_0^2 \{1 + \cos(2\zeta_\eta)\}$$
$$+ \frac{a_0}{a_\eta} \sum_l a_l a_{\eta-l} \cos(\Delta_l + \Delta_{\eta-l} - \Delta_\eta) \{2\cos(\zeta_{\eta-l} - \zeta_\eta - \zeta_l) + \cos(\zeta_{\eta-l} - \zeta_\eta + \zeta_l)\}.$$

To lowest non-zero order in $\zeta_{\eta\neq 0}$, this equation becomes

$$\dot{\zeta}_\eta = -\frac{1}{a_0} F_\mathrm{p} \sin(\phi_\mathrm{P} - \phi_0) + \frac{1}{2} d_2 \eta^2 + a_0^2 \{1 + \cos(-2\zeta_\eta)\}.$$

This equation is separable and can be integrated directly. Separation of $\zeta_\eta$ and $\tau$ yields

$$\int_{\bar{\phi}_\mu(\tau_0)-\phi_0}^{\bar{\phi}_\mu(\tau)-\phi_0} \frac{\mathrm{d}\zeta_\eta}{1 + C(\eta) + \cos(2\zeta_\eta)} = {a_0}^2 \int_{\tau_0}^{\tau} \mathrm{d}\tau',$$

where $C(\eta) = d_2\eta^2/2a_0^2 - F_\mathrm{P} \sin(\phi_\mathrm{P} - \phi_0)/a_0^3$. Integration results in

$$\frac{1}{\sqrt{C(C+2)}} \tan^{-1}\left[\sqrt{\frac{C}{C+2}} \tan\zeta_\eta\right]_{\bar{\phi}_\mu(\tau_0)-\phi_0}^{\bar{\phi}_\mu(\tau)-\phi_0} = {a_0}^2(\tau - \tau_0),$$

which can be written as

$$\tan[\bar{\phi}_\mu(\tau) - \phi_0] = \sqrt{\frac{C+2}{C}} \tan\left[\sqrt{C(C+2)}{a_0}^2(\tau - {\tau_0}')\right] \cdot$$

Here, ${\tau_0}'$ accounts for the constants of integration on both sides of the previous equality. The parameter $C \equiv C(\eta)$ appears in two combinations, $C/(C+2)$ and $C(C+2)$, which are the same insofar as the sign of what appears under the square roots is to be determined. If $-2 < C < 0$, then $C/(C+2)$ and $C(C+2)$ will be negative and the tangent on the right changes to hyperbolic tangent, i.e.

$$\tan[\bar{\phi}_\mu(\tau) - \phi_0] = \sqrt{\left|\frac{C+2}{C}\right|} \tanh\left[\sqrt{|C(C+2)|}\ |a_0|^2(\tau - {\tau_0}')\right] \cdot \tag{SM.6}$$

Because of the asymptotic behavior of $\tanh(\cdot)$ for large arguments, this expression shows that the phase averages settle to constants with respect to the phase of the pumped mode, irrespective of the initial conditions (the value of ${\tau_0}'$). We explain in the main text that this leads to phase anti-symmetrization. It is straightforward to show that the condition $-2 < C < 0$ on $C(\eta)$ is the same as the inequality ${a_0}^2 \geq |\alpha - d_2\eta^2/2 - 2{a_0}^2|$ found earlier in determining the modulational instability gain. See the discussion following Eq. (SM.5).

## The phase offset of the pumped mode with respect to the other modes in the comb

Based on Eq. (SM.6), also found in the main text, the centered average phase $\zeta_\eta = \bar{\phi}_\eta - \phi_0$ after a few units of the normalized time can be approximated by $\tan\zeta_\eta = \sqrt{|(C+2)/C|}$. For a given pump amplitude and detuning, $C = \beta\eta^2/2a_0^2 - F_\mathrm{P}\sin(\phi_\mathrm{P} - \phi_0)/a_0^3$ would be known and $\zeta_\eta$ can be calculated. For instance, for small dispersion parameter ($d_2 \ll 1$), close to the comb generation threshold ($a_0 \approx 1$), and for pumped mode phase closely following the phase of the laser mode

($\phi_{\mathrm{P}}-\phi_0 \approx 0$), $|C| \ll 1$ will hold for small mode numbers (e.g., $\eta=1$) and $\zeta_\eta$ will be close to $\pi/2$. This limit applies to the case of cavity solitons where $\eta \to 1$ makes sense. This is not usually the case for Turing rolls for which the peak of modulational instability gain may fall at a mode number much larger than $\eta=1$ (e.g., $\eta_{\max}=19$ for the example shown in Fig. 1(b) in the main text). Loh *et al.* [SM3] justify the phase offset of the pumped mode in Turing rolls based on maximizing the modulational instability gain.

## Linear stability analysis

We consider Eq. (4) in the main text for a comb with $2N+1$ phase-locked teeth. For all the indices appearing in this equation to be in the range $[-N\ ,N]$, the summation should run from $-(N-\eta)$ to $N$, i.e.,

$$\dot{\Delta}_\eta = \frac{a_0}{a_\eta}\sum\nolimits_{l=-(N-\eta)}^{N} K(l,\eta)\sin(\Delta_l+\Delta_{\eta-l}-\Delta_\eta).$$

As explained in the main text, the coupling coefficients $K$ will be the same for uniform comb magnitude spectrum. If each phase $\phi_\eta$ is perturbed from it steady-state value by $e_\eta$, the phase difference $\Delta_\eta$ will change to $\Delta_\eta+\epsilon_\eta$, where $\epsilon_\eta=(e_\eta-e_{-\eta})/2$. Plugging $\Delta_\eta+\epsilon_\eta$ into the above equation and linearizing in $\epsilon_\eta$, we find the matrix equation $\dot{\boldsymbol{\epsilon}}=K\mathbf{J}\boldsymbol{\epsilon}$ for the perturbation vector $\boldsymbol{\epsilon}=(\epsilon_1,\epsilon_2,\ldots,\epsilon_N)^{\mathrm{T}}$. The matrix $\mathbf{J}$ and its eigenvalues can be written down for general values of $N$. For odd $N$,

$$\mathbf{J}|_{N\ \mathrm{odd}} = \begin{bmatrix} -2N & 0 & \ldots & 0 & 0 & 0 & \ldots & 0 & 2 \\ 0 & -2N+1 & \ldots & \vdots & \vdots & \vdots & \ldots & 2 & 2 \\ 0 & 0 & \ldots & 0 & 0 & 0 & \ldots & 2 & 2 \\ 0 & 0 & \ldots & -2N-1+\lfloor N/2 \rfloor & 0 & 0 & \ldots & 2 & 2 \\ \vdots & \vdots & \ldots & 0 & -N+1-\lfloor N/2 \rfloor & 2 & \ldots & \vdots & \vdots \\ 0 & 0 & \ldots & 2 & 2 & -N+2-\lfloor N/2 \rfloor & \ldots & 2 & 2 \\ 0 & 0 & \ldots & 2 & 2 & 2 & \ldots & 2 & 2 \\ 0 & 2 & \ldots & \vdots & \vdots & \vdots & \ldots & -N & 2 \\ 2 & 2 & \ldots & 2 & 2 & 2 & \ldots & 2 & -N+1 \end{bmatrix},$$

and it eigenvalues are $0, -N-1, -N-2, \ldots, -N+1-\lfloor N/2 \rfloor, -N-\lfloor N/2 \rfloor, -2N-2+\lfloor N/2 \rfloor$, $-2N-3+\lfloor N/2 \rfloor, \ldots, -2N, -2N-1$. Here $\lfloor \cdot \rfloor$ is the floor function. For even $N$,

$$\mathbf{J}|_{N\ \mathrm{even}} = \begin{bmatrix} -2N & 0 & \ldots & 0 & 0 & \ldots & 0 & 2 \\ 0 & -2N+1 & \ldots & \vdots & \vdots & \ldots & 2 & 2 \\ 0 & 0 & \ldots & 0 & 0 & \ldots & 2 & 2 \\ 0 & 0 & \ldots & -2N-1+N/2 & 0 & \ldots & 2 & 2 \\ \vdots & \vdots & \ldots & 0 & 2 & \ldots & \vdots & \vdots \\ 0 & 0 & \ldots & 2 & -N+2-N/2 & \ldots & 2 & 2 \\ 0 & 0 & \ldots & 2 & 2 & \ldots & 2 & 2 \\ 0 & 2 & \ldots & \vdots & \vdots & \ldots & -N & 2 \\ 2 & 2 & \ldots & 2 & 2 & \ldots & 2 & -N+1 \end{bmatrix}.$$

And the eigenvalues of this matrix are $0, -N-1, -N-2, \ldots, -N+2-N/2\,, -N+1-N/2\,, -2N-2+N/2\,,\ -2N-3+N/2\,, \ldots, -2N, -2N-1$.

## References for the Supplemental Material

[SM1] C. Godey, I. V. Balakireva, A. Coillet, and Y. K. Chembo, “Stability analysis of the spatiotemporal Lugiato-Lefever model for Kerr optical frequency combs in the anomalous and normal dispersion regimes,” Physical Review A **89**, no. 6 (2014).

[SM2] H. Taheri, A. A. Eftekhar, K. Wiesenfeld, and A. Adibi, “Anatomy of Phase Locking in Parametric Frequency Combs,” In *Laser Science*, JW2A-12. Optical Society of America, 2015.

[SM3] W. Loh, P. Del'Haye, S. B. Papp, and S. A. Diddams, “Phase and coherence of optical microresonator frequency combs,” Physical Review A **89**, no. 5 (2014).
